# Supplementary material for: Can ChatGPT replace StackOverflow? A Study on Robustness and Reliability of Large Language Model Code Generation
Source: arXiv:2308.10335 source file (2024-01-27)
Supplement: Supplementary file 1 [file 7-appendix.tex]

\section*{Appendix}
\section{Rules Checked in \dataset{}}
% \twocolumn
The API usage patterns checked in \dataset{} are shown in Table~\ref{tab:pattern}. It is summarized based on the existing research on API misuses~\cite{zhang2018code}. Each pattern contains a sequence of control structures and method calls, separated by commas, which will be retrieved by the API usage checker and compare against the AST of code snippets. 

To be more specific, \texttt{arg0} is a variable that indicates the first argument of the function call. \texttt{rcv} is also a variable corresponding to the object of the method call. \texttt{a@C} indicates that API \texttt{a} can only be invoked when condition \texttt{C} is satisfied. 

For example, the pattern of \texttt{JsonElement.getAsString}:
\begin{align*}
\small
    \texttt{try,getAsString()@rcv!=null,end,catch(Exception),end}
\end{align*}
indicates the API \texttt{JsonElement.getAsString} can be used only when the object of \texttt{getAsString()} is valid, and the API call should be enclosed within a \texttt{try-catch} block to handle potential exceptions.

More detailed explanation of each API usage rules is as follows.
\begin{enumerate}
\small
    \item \textbf{FileChannel.write:} Execute write() within a try-catch block to handle exceptions.

    \item \textbf{FileChannel.write:} Execute write() within a try-catch for handling exceptions.

    \item \textbf{FileChannel.write/close:} To execute close()
        after write(), handling exceptions.

    \item \textbf{Activity.setContentView:} Ensure that setContentView(View)
        is called after onCreate(Bundle).

    \item \textbf{List.get:} Loop over the get(int) call while arg0 is less than
        the instance's size().

    \item \textbf{RandomAccessFile.write/close:} Execute close() after execute write(byte[]), handling exceptions.

    \item \textbf{PrintWriter.write:} Execute write(String) within try-catch for
        handling exceptions.

    \item \textbf{PrintWriter.write/close:} Execute close() after
        write(String) within try-catch for handling exceptions.

    \item \textbf{TypedArray.getString:} After calling getString(int), make
        sure to call recycle().

    \item \textbf{StringTokenizer.nextToken:} Call hasMoreTokens() to check before calling nextToken().

    \item \textbf{Map.get:} Compare the return value of get().

    \item \textbf{File.createNewFile:} Execute
        createNewFile() within try-catch for handling exceptions.

    \item \textbf{SQLiteDatabase.query:} After executing query(),
        make sure to call close().

    \item \textbf{JsonElement.getAsString:} Execute getAsString() within try-catch. Check the object is not null.

    \item \textbf{JsonElement.getAsString:} Execute getAsString() within try-catch block. Check the object with isJsonPrimitive().

    \item \textbf{String.getBytes:} Execute getBytes() within try-catch for handling exceptions.

    \item \textbf{ProgressDialog.dismiss:} Check the object of dismiss() against null.

    \item \textbf{Cipher.init:} Execute init() within try-catch for handling
        exceptions.

    \item \textbf{Cipher.init:} Execute init() before getInstance() and within try-catch for handling exceptions.

    \item \textbf{File.mkdirs:} Call exists() before create a directory using mkdirs().

    \item \textbf{ApplicationInfo.loadIcon:} Execute loadIcon() within try-catch for
        handling exceptions.

    \item \textbf{ApplicationInfo.loadIcon:} Call getPackageManager() before execute loadIcon().

    \item \textbf{BufferedReader.readLine:}  Execute readLine() within try-catch for
        handling exceptions.

    \item \textbf{BufferedReader.readLine:} Create a BufferedReader before
        execute readLine().

    \item \textbf{BufferedReader.readLine:}  Create a BufferedReader before execute
        readLine() within try-catch for handling exceptions.

    \item \textbf{BufferedReader.readLine:}  Execute readLine() within try-catch and handle Exception.
    \item \textbf{Iterator.next:} Call next() as long as the instance's hasNext() is true.

\end{enumerate}

\onecolumn
% Table generated by Excel2LaTeX from sheet 'Sheet2'
\begin{table}[!b]
  \centering
  \caption{API usage patterns checked in \dataset{}. }
    \small
\resizebox{\linewidth}{!}{
    \setlength{\tabcolsep}{2mm}{
% Table generated by Excel2LaTeX from sheet 'Sheet2'
\begin{tabular}{cll}
\toprule
      & \textbf{API} & \textbf{Pattern} \\
\midrule
1     & FileChannel.write & \texttt{try, write(ByteBuffer), end, catch(Exception), end} \\
2     & FileChannel.write & \texttt{try, getChannel(), write(ByteBuffer), end, catch(Exception), end} \\
3     & FileChannel.write/close & \texttt{try, write(ByteBuffer), close(), end, catch(Exception), end} \\
4     & Activity.setContentView & \texttt{onCreate(Bundle), setContentView(View)} \\
5     & List.get & \texttt{LOOP, get(int)@arg0<rcv.size(), end} \\
6     & RandomAccessFile.write/close & \texttt{try, write(byte[]), close(), end, catch(Exception), end} \\
7     & PrintWriter.write & \texttt{try, write(String), end, catch(Exception), end} \\
8     & PrintWriter.write/close & \texttt{try, write(String), close(), end, catch(Exception), end} \\
9     & TypedArray.getString & \texttt{getString(int), recycle()} \\
10    & StringTokenizer.nextToken & \texttt{StringTokenizer.nextToken} \\
11    & Map.get & \texttt{get(String), IF, end} \\
12    & File.createNewFile & \texttt{try, createNewFile(), end, catch(Exception), end} \\
13    & SQLiteDatabase.query & \texttt{query(String,String[],String,String[],String,String,String), close()} \\
14    & JsonElement.getAsString & \texttt{try, getAsString()@rcv!=null, end, catch(Exception), end} \\
15    & JsonElement.getAsString & \texttt{try, getAsString()@rcv.isJsonPrimitive(), end, catch(Exception), end} \\
16    & String.getBytes & \texttt{getBytes(String)} \\
17    & ProgressDialog.dismiss & \texttt{IF, dismiss()@rcv!=null, end} \\
18    & Cipher.init & \texttt{try, init(int,Key), end, catch(Exception), end} \\
19    & Cipher.init & \texttt{try, getInstance(String), init(int,Key), end, catch(Exception), end} \\
20    & File.mkdirs & \texttt{exists(), mkdirs()} \\
21    & ApplicationInfo.loadIcon & \texttt{try, loadIcon(PackageManager), end, catch(Exception), end} \\
22    & ApplicationInfo.loadIcon & \texttt{getPackageManager(), loadIcon(PackageManager)} \\
23    & BufferedReader.readLine & \texttt{try, readLine(), end, catch(Exception), end} \\
24    & BufferedReader.readLine & \texttt{new BufferedReader(InputStreamReader), readLine()} \\
25    & BufferedReader.readLine & \texttt{try, new BufferedReader(InputStreamReader), readLine(), end, catch(Exception), end} \\
26    & BufferedReader.readLine & \texttt{try, readLine(), end, catch(IOException), end} \\
27    & Iterator.next & \texttt{next()@rcv.hasNext()} \\
\bottomrule
\end{tabular}%
}}
  \label{tab:pattern}%
\end{table}%
